# Supplementary material for: HyPFuzz: Formal-Assisted Processor Fuzzing
Source: arXiv:2304.02485 source file (2023-06-24)
Supplement: Supplementary file 1 [file appendix.tex]

module code_cov_example (input a,b,c,output d);
    reg [1:0] state_d,state_q;
    always@(*)begin
        case (start_q) begin
            IDLE: begin // FSM
                if (a || b && c) begin // branch, condition
                    state_d = FINISH;
                end else begin
                    state_d = a & c; // expression
                end
            end
            ...
            FINISH: begin // FSM
                d = 1'b1; // toggle
            end
        endcase
    end
endmodule
